# Supplementary material for: Control of traveling localized spots
Source: arXiv:1703.04246 ancillary file (2018-09-20)
Supplement: Supplementary file 1 [file SI_manuscript_NJP_18-09-18.pdf]

# Supplementary Information: Control of traveling localized spots

**S. Martens[1], C. Ryll[2], J. Löber[1,3], F. Tröltzsch[2], and H. Engel[1]**

[1] Institut für Theoretische Physik, Hardenbergstraße 36, EW 7-1, Technische Universität Berlin, 10623 Berlin, Germany

[2] Technische Universität Berlin, Institut für Mathematik, Str. d. 17. Juni 136, MA 4-5, 10623 Berlin, Germany

[3] Max-Planck-Institut für Physik komplexer Systeme, Nöthnitzer Straße 38, 01187 Dresden, Germany

E-mail: steffen.martens@tu-berlin.de

## S1. Details on numerical methods

In our numerical simulations, the state equation

$$\partial_t \mathbf{U}(\mathbf{r},t) - \mathbb{D}\Delta\mathbf{U}(\mathbf{r},t) - \mathbf{R}(\mathbf{U}(\mathbf{r},t)) = \mathbf{f}(\mathbf{r},t), \tag{S1a}$$

is solved on a rectangular domain $\Omega = (x_a, x_b] \times (y_a, y_b]$ with periodic boundary conditions

$$\begin{aligned} \mathbf{U}(x_a,y,t) &= \mathbf{U}(x_b,y,t), \qquad \frac{\partial^l}{\partial^l x}\mathbf{U}(x_a,y,t) = \frac{\partial^l}{\partial^l x}\mathbf{U}(x_b,y,t),\\ \mathbf{U}(x,y_a,t) &= \mathbf{U}(x,y_b,t), \qquad \frac{\partial^l}{\partial^l y}\mathbf{U}(x,y_a,t) = \frac{\partial^l}{\partial^l y}\mathbf{U}(x,y_b,t),\ l \geq 1. \end{aligned} \tag{S1b}$$

Here, $\mathbf{U}(\mathbf{r},t) = (u_1(\mathbf{r},t),\dots,u_n(\mathbf{r},t))^T$ is the vector of $n \in \mathbb{N}$ state components defined in the two-dimensional spatial domain $\Omega \subset \mathbb{R}^2$ with $\mathbf{r} = (x,y)^T$. Further, $\mathbf{R}(\mathbf{U}) = (R_1(\mathbf{U}),\dots,R_n(\mathbf{U}))^T$ describes the reaction kinetics of the components and the $n \times n$ matrix of diffusion coefficients $\mathbb{D}$ is diagonal and constant (isotropic media), $\mathbb{D} = \mathrm{diag}(D_1,\dots,D_n)$. On the right hand side of (S1a), the space-time dependent control signals are denoted by $\mathbf{f}(\mathbf{r},t) = (f_1(\mathbf{r},t),\dots,f_m(\mathbf{r},t))^T$, $m \in \mathbb{N}$.
Without loss of generality, we fix the spots' direction of motion to coincide with the $x$-axis, i.e., $v_0^x \neq 0$ and $v_0^y = 0$. Any numerical simulation to equation (S1a) are initialized with the profile $\mathbf{U}_c$. The latter and the natural velocity $\mathbf{v}_0$ are obtained by solving the nonlinear eigenvalue problem

$$\mathbf{0} = \mathbb{D}\Delta_{\boldsymbol{\xi}}\mathbf{U}_c(\boldsymbol{\xi}) + \mathbf{v}_0 \cdot \nabla_{\boldsymbol{\xi}}\mathbf{U}_c(\boldsymbol{\xi}) + \mathbf{R}(\mathbf{U}_c(\boldsymbol{\xi})), \tag{S2}$$

with adequate accuracy.

*Simulations based on the Goldstone mode control* $\mathbf{f}_{\mathrm{Gold}}$

In all position control examples based on Goldstone mode control, we numerically solve (S1) with spectral method [1]. Transforming (S1a) into the Fourier space, one gets for the $n$-th state component

$$\frac{\partial}{\partial t}\hat{u}_n(\mathbf{k},t) = -D_n\,\mathbf{k}^2\,\hat{u}_n(\mathbf{k},t) + \mathcal{F}\{R_n(\mathbf{U}) + f_n(\mathbf{U},t)\}, \tag{S3}$$

where $\hat{u}_n$ denotes the Fourier transform $\mathcal{F}\{\cdot\}$ of the $n$-th component, $\hat{u}_n(\mathbf{k},t) = \mathcal{F}\{u_n(\mathbf{r},t)\}$, and $\mathbf{k} = (k_x,k_y)^T$ is the wave vector. Multiplying (S3) by the integrating factor $\mathrm{e}^{-c_n t}$ with $c_n = D_n\mathbf{k}^2$ and integrating the equation over a single time step from $t_m$ to $t_{m+1} = t_m + dt$, one derives the exponential time differencing (ETD) methods

$$\begin{aligned} \hat{u}_n(\mathbf{k},t_{m+1}) = {}& \hat{u}_n(\mathbf{k},t_m)\mathrm{e}^{c_n dt}\\ &+ \mathrm{e}^{c_n dt}\int_0^{dt} \mathrm{d}\tau\,\mathrm{e}^{-c_n\tau}\mathcal{F}\{R_n(\mathbf{U}(t_m+\tau),t_m+\tau) + f_n(\mathbf{U}(t_m+\tau),t_m+\tau)\}. \end{aligned} \tag{S4}$$

This formula is exact. The essence of ETD methods is in deriving approximations to the integral in this expression. In particular, we use ETD2 implying that $\mathcal{F}\{g(\mathbf{U}(t_m+$

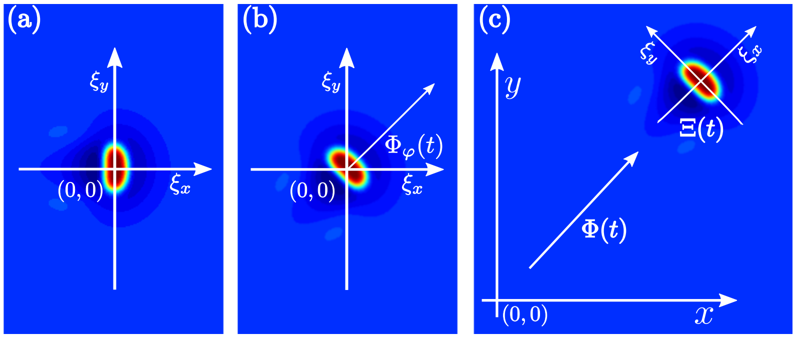


**Figure S1.** Position and orientation of the desired distribution $\mathbf{U}_d(\mathbf{r},t) = \mathbf{U}_c(\mathbb{A}(-\Phi_\varphi(t))\,(\mathbf{r}-\mathbf{\Phi}(t)))$. (a) Wave profile of the activator distribution $u_c(\boldsymbol{\xi})$ centered in the co-moving and co-rotating frame of reference at $\boldsymbol{\xi} = (0,0)^T$. (b) Counter-clockwise rotation of $u_c(\boldsymbol{\xi})$ according to the desired orientation $\Phi_\varphi(t)$. (c) Shift of the rotated solution in virtue of the translational protocol of motion $\mathbf{\Phi}(t) = (\Phi_x(t), \Phi_y(t))^T$.

$\tau), t_m+\tau)\} = \mathcal{F}\{g(\mathbf{U}(t_m),t_m)\} + \tau\left(\mathcal{F}\{g(\mathbf{U}(t_m),t_m)\} - \mathcal{F}\{g(\mathbf{U}(t_{n-1}),t_{n-1})\}\right)/dt + \mathcal{O}(dt^2)$. Finally, one arrives at the numerical scheme for ETD2

$$\begin{aligned}\hat{u}_n(\mathbf{k},t_{m+1}) &= \hat{u}_n(\mathbf{k},t_m)\mathrm{e}^{c_n dt} + \\ &+\mathcal{F}\{R_n(\mathbf{U}(t_m),t_m) + f_n(\mathbf{U}(t_m),t_m)\}\frac{\left((1+c_n\,dt)\mathrm{e}^{c_n dt} - 2\,c_n\,dt - 1\right)}{c_n^2\,dt} + \\ &+\mathcal{F}\{R_n(\mathbf{U}(t_{m-1}),t_{m-1}) + f_n(\mathbf{U}(t_{m-1}),t_{m-1})\}\frac{\left(1+c_n\,dt - \mathrm{e}^{c_n dt}\right)}{c_n^2\,dt},\end{aligned} \tag{S5}$$

which has a local truncation error of $\mathcal{O}(5\,dt^3\,\ddot{\mathcal{F}}\{\cdot\}/12)$ [1]. To avoid interpolation errors due to discretization of the spatial domain, both the desired solution $\mathbf{U}_d(\mathbf{r},t) = \mathbf{U}_c(\mathbb{A}(-\Phi_\varphi(t))\,(\mathbf{r}-\mathbf{\Phi}(t)))$ and $\mathbf{f}_{\mathrm{Gold}}$

$$\mathbf{f}_{\mathrm{Gold}}(\mathbf{r},t) = \left[\left(\begin{pmatrix} v_0^x \\ v_0^y \\ 0\end{pmatrix} - \mathbb{A}_z\left(-\Phi_\varphi(t)\right)\begin{pmatrix}\dot{\Phi}_x(t)\\ \dot{\Phi}_y(t) \\ \dot{\Phi}_\varphi(t)\end{pmatrix}\right)\cdot\tilde{\nabla}_{\boldsymbol{\xi}}\right]\mathbf{U}_c(\boldsymbol{\xi})\Bigg|_{\boldsymbol{\xi}=\mathbb{A}(-\Phi_\varphi(t))(\mathbf{r}-\mathbf{\Phi}(t))}, \tag{S6}$$

are computed with spectral methods ‡. First, the uncontrolled spot profile $\mathbf{U}_c(\mathbf{r})$ is rotated around $(0,0)^T$ in the spatial domain by $\Phi_\varphi(t)$, see figure S1(b). In a second step, the shift as given by the translational POM $\mathbf{\Phi}(t) = (\Phi_x(t), \Phi_y(t))^T$, cf. figure S1(c), is computed in Fourier space by multiplying the Fourier transform of the previously rotated spot solution with $\exp\left(-i\mathbf{k}\cdot\mathbf{\Phi}(t)\right)$, followed by the inverse Fourier transform $\mathcal{F}^{-1}\{\cdot\}$.

Analogously, we calculate $\mathbf{f}_{\mathrm{Gold}}$: First, the derivatives with respect to $x$ and $y$ are obtained numerically in Fourier space using $\partial_x\mathbf{U}_c = \mathcal{F}^{-1}\{ik_x\mathcal{F}\{\mathbf{U}_c\}\}$ and $\partial_y\mathbf{U}_c = \mathcal{F}^{-1}\{ik_y\mathcal{F}\{\mathbf{U}_c\}\}$, respectively. The angular derivative is given as the linear combination $\partial_\varphi\mathbf{U}_c = -y\partial_x\mathbf{U}_c + x\partial_y\mathbf{U}_c$. Second, all derivatives are rotated according to the orientational POM $\Phi_\varphi(t)$, followed by a shift computed in Fourier space.

‡ $\mathbb{A}(\alpha) = [\cos(\alpha), -\sin(\alpha); \sin(\alpha), \cos(\alpha)]$ denotes the clockwise rotation matrix in 2D and $\mathbb{A}_z(\alpha)$ is the clockwise rotation matrix around the $z$-axes in 3D, $\mathbb{A}_z(\alpha) = \mathrm{diag}(\mathbb{A}(\alpha), 1)$

In all simulations using ETD2, the squared domain $\Omega = (-0.5, 0.5] \times (-0.5, 0.5]$ is discretized into $256 \times 256$ spatial grid points and Fourier modes, respectively. We emphasize that the domain size is chosen sufficiently large to avoid self-interaction of the spots in the periodic simulation domain. The numerical time step $dt$ is adjusted such that the local truncation error is less than $10^{-4}$ for any protocol of motion. But $dt$ is always less than equal to $dt \leq 0.01$.

*Numerical calculation of optimal control*

For optimal control, both the state equation (S1) and the adjoint equation

$$-\partial_t \mathbf{P}(\mathbf{r}, t) - \mathbb{D}\Delta\mathbf{P}(\mathbf{r}, t) - \mathcal{D}\mathbf{R}^T(\mathbf{U}_{\text{opt}}(\mathbf{r}, t))\mathbf{P}(\mathbf{r}, t) = \mathbf{U}_{\text{opt}} - \mathbf{U}_d \quad \text{in} \quad Q, \tag{S7}$$

have to be computed. The *adjoint state* $\mathbf{P}$ has to obey the terminal condition $\mathbf{P}(\cdot, T) = \mathbf{0}$ in $\Omega$ at final time $T$ and periodic boundary conditions in $\partial\Omega$. In equation (S7), $\mathcal{D}\mathbf{R}^T$ denotes the transposed Jacobian matrix of $\mathbf{R}$ with respect to $\mathbf{U}$. The solution to the optimal control problem is determined by

$$\mathbf{P} + \nu\, \mathbf{f}_{\text{opt}} = \mathbf{0}. \tag{S8}$$

Due to the mixed initial and terminal conditions for $\mathbf{U}$ and $\mathbf{P}$ it is rarely possible to find numerical solutions to optimal control by a direct integration method. To reduce numerical costs, we employ Model Predictive Control and divide our optimal control problem into subproblems with a 4 time-step small time-horizon [2]. Thereby, each subproblem is solved with a gradient-type method which proceeds as follows: Starting for $k = 1$ with an initial guess $\mathbf{f}_{k-1} \equiv \mathbf{f}_0$ for the control, we compute $\mathbf{U}_k$ as the solution to (S1) as well as $\mathbf{P}_k$ as the solution to (S7) with $\mathbf{U}_k$ substituted for $\mathbf{U}_{\text{opt}}$. The gradient of the non-negative tracking-type functional $J$ with respect to $\mathbf{f}$, $\mathbf{d}_k$, is calculated as $\mathbf{d}_k = \mathbf{P}_k + \nu\, \mathbf{f}_{k-1}$ whereby $-\mathbf{d}_k$ defines the direction of steepest descent in function space. A new control $\mathbf{f}_k$ is iteratively obtained by

$$\mathbf{f}_k := \mathbf{f}_{k-1} - s\, \mathbf{d}_k, \tag{S9}$$

where $s$ denotes a suitable step size [3, 4]. If $\mathbf{d}_k$ satisfies an appropriately chosen termination condition, in our work this is set to $\|\mathbf{d}_k\| < 10^{-8}$, then the algorithm stops and $\mathbf{f}_k$ is identified with $\mathbf{f}_{\text{opt}}$. Otherwise, the steps are repeated iteratively for $k := k + 1$. Because the convergence of a gradient-type method can be fairly slow, the maximum number of iterations has been limited to $N_{\text{iter}} = 50$. Moreover, we keep the Tikhonov-regularization parameter fixed at $\nu = 10^{-7}$.

Many modifications of the basic algorithm sketched above exist and often lead to a better performance, as e.g. the nonlinear conjugate gradient method [5]. However, all iterative algorithms require multiple solutions of state and adjoint state equation, resulting in a rapidly increasing computational cost of numerical optimal control with the number of spatial dimensions and the length of the time interval. Therefore, the domain $\Omega$ is discretized by 256 grid points in each direction with spatial step sizes of $dx = dy = 1/256$ and the Laplacian $\Delta$ is approximated by a 5-point stencil. Due to significant computational cost of the gradient-type algorithm, we choose a moderate temporal resolution of $dt = 0.1$. For maximum stability the time evolution is computed with an implicit Euler method.

*Error estimation*

While the numerical evaluation of $\mathbf{f}_{\text{Gold}}$ is limited by the accuracy of the first spatial derivatives $\tilde{\nabla}_{\boldsymbol{\xi}}\mathbf{U}_c$, the numerical computations of $\mathbf{f}_{\text{opt}}$ is affected by errors arising both in the discretization of space and time. We stress that $\mathbf{f}_{\text{Gold}}$ is calculated using spectral differentiation, while we have to use finite difference stencils for the simulation of both the state (S1) and adjoint equation (S7) in order to reduce computational costs. Nevertheless, the limiting error arises from the time step chosen in the implicit Euler-scheme. Despite that the latter is A-stable, the local truncation error is $\mathcal{O}(dt^2)$ and the error at a specific time $t$ is of the order of $\mathcal{O}(dt)$. Consequently, one observes that the relative error $\|f_{u,\text{Gold}}(t) - f_{u,\text{opt}}(t)\|_{L^1(\Omega)}$ is bounded from above by $dt$.

*Simulation times*

As already mentioned, optimal control algorithm requires much more computational resources compared to the analytic expression $f_{\text{Gold}}$. For instance, the computation of optimal position control along the Lissajous curve, see figure 4 in the main manuscript, with a short period of $T = 200$, i.e., 2000 time iterations steps with $dt = 0.1$, takes roughly 50 hours by using 3 cores (Intel i5 − 6500 with 3.20GHz) in parallel. Contrary, the same numerical simulation of (S1) based on $\mathbf{f}_{\text{Gold}}$ runs approximately one hour on the same PC. The relatively short simulation times enable us not only to use integration schemes with smaller numerical truncation error, e.g., spectral methods with ETD2 [1], but also to move the spot along longer, more complex trajectories [SI_video2,SI_video3].

## S2. Interaction of traveling spot solution with a circular heterogenity of jump type

We realize a local heterogeneity in the medium by a circular defect of jump type (step-function) in the additive parameter $\kappa_1$:

$$\kappa_1(\mathbf{r}) = \begin{cases} \kappa_1^{\text{back}}, & \forall \mathbf{r} \notin \Omega_\circ, \\ \kappa_1^{\text{het}}, & \forall \mathbf{r} \in \Omega_\circ. \end{cases} \tag{S10}$$

Thereby, the circular domain with radius $R$ is centered at $(0,0)$ and is defined by $\Omega_\circ = \{(x,y) \in \mathbb{R}^2 : x^2 + y^2 < R^2\}$.

In order to make a collision experiment, we initiate one spot moving rightwards ($v_0^x > 0$) at the far left edge of the simulation domain and measure the response to a circular defect with radius $R = 0.1$ located at $(0,0)$. The outcomes of collisions are classified as in the phase diagram of figure S2 depending on the difference $\epsilon$ between the constant background value $\kappa_1^{\text{back}}$ and $\kappa_1^{\text{het}}$ inside the heterogeneity, $\epsilon = \kappa_1^{\text{het}} - \kappa_1^{\text{back}}$. For the parameter set 1 in table 1 with $\kappa_1^{\text{back}} = -6.92$, one observes three qualitatively different regimes: splitting, transmission, and nucleation of new spots, figure S2(a). If $\kappa_1^{\text{het}}$ is smaller than the background value, the single initiated spot splits into two when reaching the left edge of the heterogeneity. Thereby, the initial velocity vector is conserved. Increasing the value of $\kappa_1^{\text{het}}$ and thus decreasing the difference $\epsilon$, the spot is able to pass the defect. With growing difference $\epsilon$, spots first enter the defect and split into multiple solutions when leaving the obstacle at the right edge. Further increasing the difference results in multiple creation of spots inside the defect. For $\kappa_1^{\text{het}} \gg \kappa_1^{\text{back}}$, the spot is able to enter the defect, gets trapped inside, and initiates the creation of multiple spots.

The observed scenarios of spot-defect-interactions are different for the second parameter set in table 2 and $\kappa_1^{\text{back}} = -7.30$. There, one discovers three qualitatively different regimes: trapping, transmission, and reflection, figure S2(b). For $\kappa_1^{\text{het}} \ll \kappa_1^{\text{back}}$, the spot pins at the outer edge of the defect and starts to move around the heterogeneity. With shrinking difference $\epsilon$, the spot gets first reflected for $\kappa_1^{\text{het}} < \kappa_1^{\text{back}}$, then is able to pass the defect for $\epsilon \approx 0$, and eventually gets trapped inside the heterogeneity for $\epsilon \in [0.09, 0.26]$. In the last scenario, the trapped spot eventually performs circular motion at the inside of the defect. A further increase of $\kappa_1^{\text{het}}$ results in various reflection scenarios.

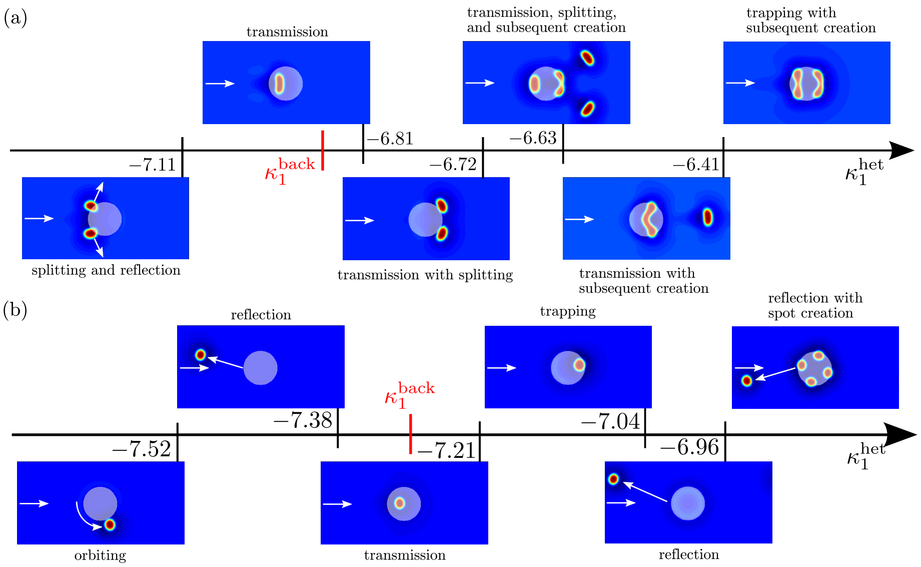


**Figure S2.** Interaction outcomes of a traveling spot with a circular defect (light blue). (a) Splitting and different regimes of transmission or nucleation of new spots [SI_video1]. Parameter set 1 in Table 1 (main manuscript) with $\kappa_1^{back} = -6.92$. (b) Trapping, reflection, transmission, and nucleation of new spots. Parameter set 2 in Table 1 (main manuscript) with $\kappa_1^{back} = -7.30$: Shown are snapshots of the activator distribution in a rectangular spatial domain of size $\Omega = [0, 1) \times [-0.25, 0.25)$ with periodic boundary conditions. Simulations were performed using ETD2 in time, cf. section S1.

## S3. Asymptotic perturbation analysis – projection method

We presume that the uncontrolled reaction-diffusion system (S1a) possesses a stable traveling wave (TW) solution $\mathbf{U}_c$ which either propagates smoothly with velocity $\mathbf{v}_0 = (v_0^x, v_0^y)^T$ or rotates around its center of rotation with angular velocity $\omega_0$. Such a pattern satisfies

$$\mathbf{0} = \mathbb{D}\Delta_{\boldsymbol{\xi}}\mathbf{U}_c(\boldsymbol{\xi}) + \omega_0\partial_{\tilde{\varphi}}\mathbf{U}_c(\boldsymbol{\xi}) + (\mathbb{A}(-\omega_0 t)\mathbf{v}_0)\cdot\nabla_{\boldsymbol{\xi}}\mathbf{U}_c(\boldsymbol{\xi}) + \mathbf{R}(\mathbf{U}_c(\boldsymbol{\xi})), \qquad \text{(S11)}$$

in the frame of reference $\boldsymbol{\xi} \equiv (\xi_x, \xi_y)^T = \mathbb{A}(-\omega_0 t)(\mathbf{r} - \mathbf{v}_0 t)$ co-moving with the velocity $\mathbf{v}_0$ and co-rotating with angular frequency $\omega_0$. Here, $\mathbb{A}(\alpha) =$

$[\cos(\alpha)\,, -\sin(\alpha); \sin(\alpha)\,, \cos(\alpha)]$ is the clockwise rotation matrix in 2D. In the co-moving coordinates $\boldsymbol{\xi}$, the angular derivative is given by $\partial_{\tilde{\varphi}} = -\xi_y \partial_{\xi_x} + \xi_x \partial_{\xi_y}$. Obviously, (S11) depends explicitly on time $t$ if the TW pattern simultaneously moves and rotates, $\omega_0 \mathbf{v}_0 \neq \mathbf{0}$. Consequently, we have to claim that the considered pattern either move, solely rotate, or is at rest, i.e., $|\mathbf{v}_0| = \omega_0 = 0$. In what follows, we keep both characteristic quantities in our derivations but always have in mind that at least one of them must be zero.

*Goldstone modes and response functions*

The stability of the TW pattern $\mathbf{U}_c$ is determine by the eigenvalues of the linear stability operator $\mathcal{L}$. The latter arises by expanding (S11) around $\mathbf{U}_c$

$$\mathcal{L} = \mathbb{D}\Delta_{\boldsymbol{\xi}} + \omega_0 \partial_{\tilde{\varphi}} + (\mathbb{A}(-\omega_0 t)\mathbf{v}_0) \cdot \nabla_{\boldsymbol{\xi}} + \mathcal{D}\mathbf{R}(\mathbf{U}_c\,(\boldsymbol{\xi})), \tag{S12}$$

in the frame of reference $\boldsymbol{\xi}$. Thereby, $\mathcal{D}\mathbf{R}\,(\mathbf{U}_c)$ denotes the Jacobian matrix of $\mathbf{R}$ evaluated at $\mathbf{U}_c$. Since we presume that $\mathbf{U}_c(\boldsymbol{\xi})$ is stable, the eigenvalue of $\mathcal{L}$ with the largest real part is $\lambda_0 = 0$ and the corresponding eigenfunctions $\mathbf{W}_i(\boldsymbol{\xi})$, $i \in \{\xi_x, \xi_y, \tilde{\varphi}\}$, also called the *propagator modes*, can be expressed by the Goldstone modes $\partial_i \mathbf{U}_c(\boldsymbol{\xi})$, $i \in \{\xi_x, \xi_y, \tilde{\varphi}\}$ . Calculating the derivative of (S11) with respect to $\xi_x$, $\xi_y$, and $\tilde{\varphi}$, one gets

$$0 = \mathcal{L}\partial_{\xi_x}\mathbf{U}_c(\boldsymbol{\xi}) + \omega_0\, \partial_{\xi_y}\mathbf{U}_c(\boldsymbol{\xi}), \tag{S13a}$$
$$0 = \mathcal{L}\partial_{\xi_y}\mathbf{U}_c(\boldsymbol{\xi}) - \omega_0\, \partial_{\xi_x}\mathbf{U}_c(\boldsymbol{\xi}), \tag{S13b}$$
$$0 = \mathcal{L}\partial_{\tilde{\varphi}}\mathbf{U}_c(\boldsymbol{\xi}) - \mathbf{v}_0 \times \nabla_{\boldsymbol{\xi}}\mathbf{U}_c(\boldsymbol{\xi}). \tag{S13c}$$

These relations can be re-written in a compact form

$$\mathcal{L}\begin{pmatrix}\partial_{\xi_x}\mathbf{U}_c(\boldsymbol{\xi})\\ \partial_{\xi_y}\mathbf{U}_c(\boldsymbol{\xi})\\ \partial_{\tilde{\varphi}}\mathbf{U}_c(\boldsymbol{\xi})\end{pmatrix} = \begin{pmatrix}-\omega_0\, \partial_{\xi_y}\mathbf{U}_c(\boldsymbol{\xi})\\ \omega_0\, \partial_{\xi_x}\mathbf{U}_c(\boldsymbol{\xi})\\ \mathbf{v}_0 \times \partial_{\tilde{\varphi}}\mathbf{U}_c(\boldsymbol{\xi})\end{pmatrix} = \begin{pmatrix}0 & -\omega_0 & 0\\ \omega_0 & 0 & 0\\ v_y^0 & -v_0^x & 0\end{pmatrix}\begin{pmatrix}\partial_{\xi_x}\mathbf{U}_c(\boldsymbol{\xi})\\ \partial_{\xi_y}\mathbf{U}_c(\boldsymbol{\xi})\\ \partial_{\tilde{\varphi}}\mathbf{U}_c(\boldsymbol{\xi})\end{pmatrix}, \tag{S14}$$

The adjoint operator $\mathcal{L}^\dagger$ to $\mathcal{L}$ is defined with respect to the standard inner product in two-dimensional function space

$$\langle \mathbf{u}, \mathcal{L}\mathbf{v}\rangle = \left\langle \mathcal{L}^\dagger \mathbf{u}, \mathbf{v}\right\rangle \quad \text{with} \quad \langle \mathbf{u}, \mathbf{v}\rangle = \int\limits_{-\infty}^{\infty}\int\limits_{-\infty}^{\infty} \mathrm{d}^2\mathbf{r}\overline{\mathbf{u}}^T(\mathbf{r})\,\mathbf{v}\,(\mathbf{r})\,, \tag{S15}$$

where $\overline{\mathbf{u}}$ denotes complex conjugation; yielding

$$\mathcal{L}^\dagger = \mathbb{D}\Delta_{\boldsymbol{\xi}} - \omega_0 \partial_{\tilde{\varphi}} - (\mathbb{A}(-\omega_0 t)\mathbf{v}_0) \cdot \nabla_{\boldsymbol{\xi}} + \mathcal{D}\mathbf{R}(\mathbf{U}_c\,(\boldsymbol{\xi}))^T. \tag{S16}$$

Next, we introduce the so-called *response functions* $\mathbf{W}_i^\dagger(\boldsymbol{\xi})$, $i \in \{\xi_x, \xi_y, \tilde{\varphi}\}$. Although the latter do not coincide with the eigenfunctions of $\mathcal{L}^\dagger$ to eigenvalue zero, they are closely related to these. The response functions are also not identical to $\mathbf{W}_i$, $i \in \{\xi_x, \xi_y, \tilde{\varphi}\}$ because $\mathcal{L}$ is in general not self-adjoint. Regarding the Goldstone modes and response functions, one can distinguish three cases corresponding to (i) stationary solutions, (ii) traveling localized patterns like spots, and (iii) rotating solutions as e.g. spiral waves.

(i) For stationary, immobile solutions with $v_0^x = v_0^y = \omega_0 = 0$, all Goldstone-modes $\partial_i \mathbf{U}_c$, $i \in \{\xi_x, \xi_y, \tilde{\varphi}\}$, are ordinary eigenfunctions of $\mathcal{L}$ to eigenvalue $\lambda_0 = 0$. Additionally, the response functions are also ordinary eigenfunctions of $\mathcal{L}^\dagger$ to $\lambda_0 = 0$. For stationary patterns, $\mathcal{L}$ can be expressed by the product of a diagonal square matrix $\mathbb{M}$ and a self-adjoint matrix $\mathbb{L}$, $\mathcal{L} = \mathbb{M}\,\mathbb{L}$. Then, the eigenfunction $\mathbf{W}_i^\dagger$ are determined by the relation $\mathbf{W}_i^\dagger = \mathbb{M}^{-1}\partial_i \mathbf{U}_c$, $i \in \{\xi_x, \xi_y, \tilde{\varphi}\}$, for a given Goldstone mode $\partial_i \mathbf{U}_c$ [6].

(ii) For traveling localized patterns with $\omega_0 = 0$, both translational Goldstone modes $\partial_{\xi_x}\mathbf{U}_c$ and $\partial_{\xi_y}\mathbf{U}_c$ are ordinary eigenfunctions of $\mathcal{L}$ to $\lambda_0 = 0$. Similar, the response functions $\mathbf{W}_{\xi_x}^\dagger$ and $\mathbf{W}_{\xi_y}^\dagger$ are determined by $\mathcal{L}^\dagger \mathbf{W}_i^\dagger = 0$, $i \in \{\xi_x, \xi_y\}$. On the other hand, the rotational Goldstone mode $\partial_{\tilde{\varphi}}\mathbf{U}_c$ is a generalized eigenfunction of rank $k = 2$ to eigenvalue 0 such that $\mathcal{L}^2 \partial_{\tilde{\varphi}}\mathbf{U}_c = 0$ or $\mathcal{L}\partial_{\tilde{\varphi}}\mathbf{U}_c = v_0^y \partial_{\xi_x}\mathbf{U}_c - v_0^x \partial_{\xi_y}\mathbf{U}_c$. In a similar fashion, the corresponding rotational response function can be obtained as a solution of $\mathcal{L}^\dagger \mathbf{W}_{\tilde{\varphi}}^\dagger = v_0^y \mathbf{W}_{\xi_x}^\dagger - v_0^x \mathbf{W}_{\xi_y}^\dagger$.

(iii) In the case of solely rotating solutions with $\mathbf{v}_0 = \mathbf{0}$, only the rotational Goldstone mode $\partial_{\tilde{\varphi}}\mathbf{U}_c(\boldsymbol{\xi})$ is an usual eigenfunction of $\mathcal{L}$ to eigenvalue zero, $\mathcal{L}\partial_{\tilde{\varphi}}\mathbf{U}_c(\boldsymbol{\xi}) = 0$. The same holds for the adjoint operator and the rotational response function, i.e., $\mathcal{L}^\dagger \mathbf{W}_{\tilde{\varphi}}^\dagger(\boldsymbol{\xi}) = 0$. Although, the translational Goldstone modes $\partial_i \mathbf{U}_c$, $\{\xi_x, \xi_y\}$ are not eigenfunctions of $\mathcal{L}$, linear combinations of them, viz. $\mathbf{Y}_\mp(\boldsymbol{\xi}) = \pm i \partial_{\xi_x}\mathbf{U}_c + \partial_{\xi_y}\mathbf{U}_c$, yield eigenfunctions to eigenvalues $\lambda_{\pm 1} = \pm i\omega_0$, $\mathcal{L}\mathbf{Y}_\mp(\boldsymbol{\xi}) = \pm i\omega_0 \mathbf{Y}_\mp(\boldsymbol{\xi})$. Since eigenvalues of $\mathcal{L}$ and the adjoint operator $\mathcal{L}^\dagger$ are complex conjugate to each other, there must be corresponding eigenfunctions $\mathbf{Y}_\mp^\dagger(\boldsymbol{\xi})$ to the adjoint operator $\mathcal{L}^\dagger$, $\mathcal{L}^\dagger \mathbf{Y}_\mp^\dagger(\boldsymbol{\xi}) = \pm i\omega_0 \mathbf{Y}_\mp^\dagger(\boldsymbol{\xi})$.

*Multiple scale perturbation expansion – Asymptotic perturbation analysis*

In order to quantify the response of the stable spot pattern $\mathbf{U}_c$ to an external control $\mathbf{f}(\mathbf{U}(\mathbf{r},t),\mathbf{r},t)$ in (S1a), we perform a multiple scale perturbation expansion in the small time scale $T = \epsilon t$. The time derivative is transformed as $\partial_t \to \partial_t + \epsilon \partial_T$ and from now on $t$ and $T$ are treated as two independent variables. The state $\mathbf{U}$ is now a function of this new time scale while the perturbation $\mathbf{f}$ depends on $T$ only through $\mathbf{U}$, i.e., $\mathbf{U} = \mathbf{U}(\mathbf{r},t,T)$ and $\mathbf{f} = \mathbf{f}(\mathbf{U}(\mathbf{r},t,T),\mathbf{r},t)$. Introducing this time scale, the perturbed RDS (2a) reads as

$$\partial_t \mathbf{U}(\mathbf{r},t,T) + \epsilon \partial_T \mathbf{U}(\mathbf{r},t,T) = \mathbb{D}\Delta\mathbf{U} + \mathbf{R}(\mathbf{U}(\mathbf{r},t,T)) + \mathbb{B}\,\mathbf{f}(\mathbf{U}(\mathbf{r},t,T)\,\mathbf{r},t). \tag{S17}$$

If the perturbations $\mathbb{B}\,\mathbf{f}$ are weak, the latter mainly causes translation and rotation of the TW pattern. Thus, we define the current position and orientation by $\boldsymbol{\Phi}(t,T) = (\Phi_x(t,T), \Phi_y(t,T))^T$ and $\Phi_\varphi(t,T)$, respectively. We stress that the two depend on both time scales. Then, we can introduce the new co-moving coordinate

$$\tilde{\mathbf{r}} = \tilde{\mathbf{r}}(\mathbf{r},t,T) = \mathbb{A}(-\Phi_\varphi(t,T)) \cdot (\mathbf{r} - \boldsymbol{\Phi}(t,T)), \tag{S18}$$

which transforms (S17) into

$$\begin{aligned}\partial_t \mathbf{U}(\tilde{\mathbf{r}},t,T) + \epsilon\partial_T \mathbf{U}(\tilde{\mathbf{r}},t,T) &= \mathbb{D}\Delta\mathbf{U}(\tilde{\mathbf{r}},t,T) + \mathbf{R}(\mathbf{U}(\tilde{\mathbf{r}},t,T)) + \\ &+ \mathbb{B}\,\mathbf{f}(\mathbf{U}(\tilde{\mathbf{r}},t,T), \mathbb{A}(\Phi_\varphi(t,T))\cdot\tilde{\mathbf{r}} + \boldsymbol{\Phi}(t,T), t) + \partial_t\Phi_\varphi(t,T)\,\partial_{\tilde{\varphi}}\mathbf{U}(\tilde{\mathbf{r}},t,T) + \\ &+ (\mathbb{A}(-\Phi_\varphi(t,T))\,\partial_t\boldsymbol{\Phi}(t,T))\cdot\nabla_{\tilde{\mathbf{r}}}\mathbf{U}(\tilde{\mathbf{r}},t,T) + \epsilon\partial_T\Phi_\varphi(t,T)\,\partial_{\tilde{\varphi}}\mathbf{U}(\tilde{\mathbf{r}},t,T) + \\ &+ \epsilon(\mathbb{A}(-\Phi_\varphi(t,T))\,\partial_T\boldsymbol{\Phi}(t,T))\cdot\nabla_{\tilde{\mathbf{r}}}\mathbf{U}(\tilde{\mathbf{r}},t,T).\end{aligned} \tag{S19}$$

Now, we suppose that the perturbed solution to (S19) can be composed of the unperturbed, stable TW solution $\mathbf{U}_c$ and a function $\tilde{\mathbf{v}}$

$$\mathbf{U} = \mathbf{U}_c + \epsilon \tilde{\mathbf{v}}. \tag{S20}$$

Thereby, $\tilde{\mathbf{v}}$ is assumed to be orthogonal to the response functions $\mathbf{W}_i^\dagger$, $\langle \mathbf{W}_i^\dagger, \tilde{\mathbf{v}} \rangle = 0$. Using this ansatz, we expand the solution in orders of $\epsilon$ and get in leading order $\mathcal{O}(1)$

$$\begin{aligned} \mathbb{D}\Delta \mathbf{U}_c(\tilde{\mathbf{r}}) &+ \partial_t \Phi_\varphi(t,T)\,\partial_{\tilde{\varphi}} \mathbf{U}_c(\tilde{\mathbf{r}}) + \\ &+ \left(\mathbb{A}\left(-\Phi_\varphi(t,T)\right)\partial_t \mathbf{\Phi}(t,T)\right)\cdot \nabla_{\tilde{\mathbf{r}}} \mathbf{U}_c(\tilde{\mathbf{r}}) + \mathbf{R}\left(\mathbf{U}_c(\tilde{\mathbf{r}})\right) = 0. \end{aligned} \tag{S21}$$

From the comparison with (S11) it becomes immediately clear that the functions $\Phi_\varphi$ and $\mathbf{\Phi}$ must behave like

$$\mathbf{\Phi}(t,T) = \mathbf{v}_0 t + \mathbf{p}(T) + \mathcal{O}(\epsilon), \tag{S22}$$
$$\Phi_\varphi(t,T) = \omega_0 t + p_\varphi(T) + \mathcal{O}(\epsilon), \tag{S23}$$

with $\mathbf{p}(T) = \left(p_x(T), p_y(T)\right)^T$ and the $p_\varphi$ depend only on the slow time scale $T$. Using the last result, we get in order $\mathcal{O}(\epsilon)$

$$\begin{aligned} \partial_t \tilde{\mathbf{v}}(\tilde{\mathbf{r}},t,T) - \mathcal{L}\tilde{\mathbf{v}} =& \partial_T \Phi_\varphi(t,T)\,\partial_{\tilde{\varphi}} \mathbf{U}_c(\tilde{\mathbf{r}}) + \left(\mathbb{A}\left(-\Phi_\varphi(t,T)\right)\partial_T \mathbf{\Phi}(t,T)\right)\cdot \nabla_{\tilde{\mathbf{r}}} \mathbf{U}_c(\tilde{\mathbf{r}}) \\ &+ \mathbb{B}\,\mathbf{f}\left(\mathbf{U}_c(\tilde{\mathbf{r}},t,T), \mathbb{A}\left(\Phi_\varphi(t,T)\right)\tilde{\mathbf{r}} + \mathbf{\Phi}(t,T), t\right), \end{aligned} \tag{S24}$$

where $\mathcal{L}$ denotes the linear stability operator of $\mathbf{U}_c$, (S12). Equation (S24) is a linear PDE with an inhomogeneity on the r.h.s.. Next, we multiply from the left with one of the three response function $\mathbf{W}_i^\dagger(\tilde{\mathbf{r}})$, $i \in \{x,y,\varphi\}$ and invoke the relations $\langle \mathbf{W}_i^\dagger, \partial_t \tilde{\mathbf{v}} \rangle = \partial_t \langle \mathbf{W}_i^\dagger, \tilde{\mathbf{v}} \rangle = 0$ and $\langle \mathbf{W}_i^\dagger, \mathcal{L}\tilde{\mathbf{v}} \rangle = \langle \mathcal{L}^\dagger \mathbf{W}_i^\dagger, \tilde{\mathbf{v}} \rangle = 0$ to eliminate the l.h.s.

$$\begin{aligned} 0 =& \partial_T \Phi_\varphi(t,T)\left\langle \mathbf{W}_i^\dagger(\tilde{\mathbf{r}}), \partial_{\tilde{\varphi}} \mathbf{U}_c(\tilde{\mathbf{r}}) \right\rangle + \left(\mathbb{A}\left(-\Phi_\varphi(t,T)\right)\cdot \partial_T \mathbf{\Phi}(t,T)\right)\cdot \langle \mathbf{W}_i^\dagger(\tilde{\mathbf{r}}), \nabla_{\tilde{\mathbf{r}}} \mathbf{U}_c(\tilde{\mathbf{r}}) \rangle \\ &+ \left\langle \mathbf{W}_i^\dagger(\tilde{\mathbf{r}}), \mathbb{B}\,\mathbf{f}\left(\mathbf{U}_c(\tilde{\mathbf{r}},t,T), \mathbb{A}\left(\Phi_\varphi(t,T)\right)\tilde{\mathbf{r}} + \mathbf{\Phi}(t,T), t\right) \right\rangle. \end{aligned} \tag{S25}$$

Introducing $\mathbb{A}_z(\alpha)$ for the clockwise rotation matrix around the $z$-axes in 3D, $\mathbb{A}_z(\alpha) = [\cos(\alpha), -\sin(\alpha), 0; \sin(\alpha), \cos(\alpha), 0; 0, 0, 1]$, (S25) can be written as

$$\mathcal{C}\mathbb{A}^z\left(-\Phi_\varphi(t,T)\right)\partial_T \begin{pmatrix} \Phi_x(t,T) \\ \Phi_y(t,T) \\ \Phi_\varphi(t,T) \end{pmatrix} = -\begin{pmatrix} \langle \mathbf{W}_x^\dagger, \mathbb{B}\,\mathbf{f} \rangle \\ \langle \mathbf{W}_y^\dagger, \mathbb{B}\,\mathbf{f} \rangle \\ \langle \mathbf{W}_\varphi^\dagger, \mathbb{B}\,\mathbf{f} \rangle \end{pmatrix}, \tag{S26}$$

where $\mathcal{C}_{ij} = \langle \mathbf{W}_i^\dagger, \partial_j \mathbf{U}_c \rangle$, $i \in \{x,y,\varphi\}$.
Because any dependence on the second time scale $T$ appears only in the general position vector $\mathbf{\Xi}(t,T) = \left(\Phi_x(t,T), \Phi_y(t,T), \Phi_\varphi(t,T)\right)^T$, we can eliminate the second time scale $T$ with one last step. Therefore, we introduce the single time scale function $\mathbf{\Xi}(t) = \mathbf{\Xi}(t, \epsilon t)$, yielding $\partial_t \mathbf{\Xi}(t) = \partial_t \mathbf{\Xi}(t,T) + \epsilon \partial_T \mathbf{\Xi}(t,T)$. Finally, we derive the equations of motion for a localized TW pattern under the impact of a weak perturbation $\mathbf{f}$ using (S22), (S23), and (S26)

$$\frac{\mathrm{d}}{\mathrm{d}t}\begin{pmatrix} \Phi_x(t) \\ \Phi_y(t) \\ \Phi_\varphi(t) \end{pmatrix} = \begin{pmatrix} v_0^x \\ v_0^y \\ \omega_0 \end{pmatrix} - \epsilon \mathbb{A}^z\left(\Phi_\varphi(t)\right)\mathcal{C}^{-1}\begin{pmatrix} \langle \mathbf{W}_x^\dagger, \mathbb{B}\,\mathbf{f} \rangle \\ \langle \mathbf{W}_y^\dagger, \mathbb{B}\,\mathbf{f} \rangle \\ \langle \mathbf{W}_\varphi^\dagger, \mathbb{B}\,\mathbf{f} \rangle \end{pmatrix}, \tag{S27}$$

with

$$\langle \mathbf{W}_i^\dagger, \mathbb{B}\,\mathbf{f}\rangle = \int_{-\infty}^{\infty}\int_{-\infty}^{\infty} \mathrm{d}^2\mathbf{r}\overline{\mathbf{W}_i^\dagger}^T \left(\mathbb{A}\left(-\Phi_\varphi\left(t\right)\right)\left(\mathbf{r}-\mathbf{\Phi}\left(t\right)\right)\right)\mathbb{B}\,\mathbf{f}\left(\mathbf{r},t\right) \tag{S28}$$

*Solving for the control*

In what follows, we study the inverse problem and view (S27) as a conditional equation for the control $\mathbf{f}$. The latter is assumed to be a linear superposition of Goldstone modes

$$\epsilon\mathbb{B}\,\mathbf{f}(\mathbf{r},t) = K_1\partial_x\mathbf{U}_c\left(\boldsymbol{\xi}(t)\right) + K_2\partial_y\mathbf{U}_c\left(\boldsymbol{\xi}(t)\right) + K_3\partial_\varphi\mathbf{U}_c\left(\boldsymbol{\xi}(t)\right), \tag{S29}$$

where $\mathbf{U}_c$ is evaluated at the presumed position in space $\bar{\boldsymbol{\xi}}(t) = \mathbb{A}\left(-\Phi_\varphi\left(t\right)\right)\left(\mathbf{r}-\mathbf{\Phi}\left(t\right)\right)$. Plugging (S29) into $\left\langle \mathbf{W}_i^\dagger, \mathbb{B}\,\mathbf{f}\right\rangle$, $i\in\{x,y,\varphi\}$, one gets

$$\epsilon\begin{pmatrix}\left\langle \mathbf{W}_x^\dagger, \mathbb{B}\,\mathbf{f}\right\rangle\\ \left\langle \mathbf{W}_y^\dagger, \mathbb{B}\,\mathbf{f}\right\rangle\\ \left\langle \mathbf{W}_\varphi^\dagger, \mathbb{B}\,\mathbf{f}\right\rangle\end{pmatrix} = \mathcal{C}\begin{pmatrix}K_1\\K_2\\K_3\end{pmatrix}, \tag{S30}$$

and, hence, the expansion coefficients $K_j$ are given as

$$\begin{pmatrix}K_1\\K_2\\K_3\end{pmatrix} = \mathbb{A}^z\left(-\Phi_\varphi\left(t\right)\right)\left[\begin{pmatrix}v_0^x\\v_0^y\\\omega_0\end{pmatrix} - \frac{\mathrm{d}}{\mathrm{d}t}\begin{pmatrix}\Phi_x(t)\\\Phi_y(t)\\\Phi_\varphi(t)\end{pmatrix}\right]. \tag{S31}$$

Finally, we obtain the analytical expressions for Goldstone mode control $\mathbf{f}_{\mathrm{Gold}}$ based on asymptotic perturbation analysis

$$\mathbf{f}_{\mathrm{Gold}}(\mathbf{r},t) = \left[\left(\begin{pmatrix}v_0^x\\v_0^y\\\omega_0\end{pmatrix} - \mathbb{A}_z\left(-\Phi_\varphi(t)\right)\frac{\mathrm{d}}{\mathrm{d}t}\begin{pmatrix}\Phi_x(t)\\\Phi_y(t)\\\Phi_\varphi(t)\end{pmatrix}\right)\cdot\tilde{\nabla}_{\boldsymbol{\xi}}\right]\mathbf{U}_c(\boldsymbol{\xi})\Bigg|_{\boldsymbol{\xi}=\bar{\boldsymbol{\xi}}(t)}. \tag{S32}$$

We stress that the derivatives $\tilde{\nabla}_{\boldsymbol{\xi}}\mathbf{U}_c$, with $\tilde{\nabla}_{\boldsymbol{\xi}} = (\partial_{\xi_x}, \partial_{\xi_y}, \partial_\varphi)^T$, have to be calculated in the co-moving and co-rotation frame of reference and then evaluated at the currently presumed position of the pattern $\bar{\boldsymbol{\xi}}(t) = \mathbb{A}\left(-\Phi_\varphi\left(t\right)\right)\left(\mathbf{r}-\mathbf{\Phi}\left(t\right)\right)$.


[1] Cox S M and Matthews P C 2002 *J. Comp. Phys.* **176** 430–455 URL `http://www.sciencedirect.com/science/article/pii/S0021999102969950`

[2] Ryll C, Löber J, Martens S, Engel H and Tröltzsch F 2016 Analytical, optimal, and sparse optimal control of traveling wave solutions to reaction-diffusion systems *Control of Self-Organizing Nonlinear Systems* ed Schöll E, Klapp S H L and Hövel P (Springer) pp 189–210 ISBN 978-3-319-28028-8 URL `http://dx.doi.org/10.1007/978-3-319-28028-8_10`

[3] Hoffmann K H, Leugering G and Tröltzsch F (eds) 1998 *Optimal Control of Partial Differential Equations* (*ISNM* vol 133) (Birkhäuser Verlag)

[4] Hoffmann K H, Lasiecka I, Leugering G, Sprekels J and Tröltzsch F (eds) 2002 *Optimal Control of Complex Structures* (*ISNM* vol 139) (Birkhäuser Verlag)

[5] Buchholz R, Engel H, Kammann E and Tröltzsch F 2013 *Comput. Optim. Appl.* **56** 153–185

[6] Gurevich S, Bödeker H, Moskalenko A, Liehr A and Purwins H G 2004 *Physica D* **199** 115–128 URL `http://linkinghub.elsevier.com/retrieve/pii/S0167278904003094`
